# Supplementary material for: Measuring the Sense of Presence and Learning Efficacy in Immersive Virtual Assembly Training
Source: arXiv:2312.10387 source file (2023-12-16)

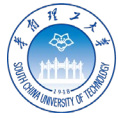

# Appendix I: Pre-test

Name \_\_\_\_\_ Gender \_\_\_\_\_  
Age \_\_\_\_\_ Studies \_\_\_\_\_

**Have you had any experience in Virtual Reality before?**

Yes ☐ No ☐

If yes, with what type of device? ☐ Mobile Device (Cardboard type)

☐ Virtual reality head mounted display (type Oculus rift, Htc Vive...) ☐ I don't know what device it was

**What is your impression of the experience in virtual reality? Just a quick description:**

\_\_\_\_\_  
\_\_\_\_\_

**Have you ever touched or used a bench machine vise? Tell me what you know about it:**

(e.g. I need a flat mouth pliers for my DIY in the lab and I know how it works...)\_\_\_\_\_

\_\_\_\_\_  
\_\_\_\_\_

**How long do you think it will take to assemble a bench vise? (Unit: min) \_\_\_\_\_**

**[ Mark with an X the box you consider correct ]**

**1. What is the main function of the bench vise?**

- ☐ Holding and securing objects
- ☐ Cutting and severing materials
- ☐ Striking and hammering objects
- ☐ Grinding and polishing surfaces

**2. What are the main components of a bench vise?**

- ☐ Vise arms, vise body, adjusting chain, movable block, screw assembly, guide assembly, pivot, spring
- ☐ Vise seat, washers, screws, jaws, movable jaws, pins, nuts, washers, screws, square nuts
- ☐ Hammerhead, handle, hook, gears, drive shaft, motor, circuit board
- ☐ Mechanical arm, sensors, controller, actuator, power supply, communication module, development board

**3. Which components can be used to adjust the clamping force and opening degree of a bench vise?**

- ☐ Pins, nuts, screws, and washers
- ☐ Pivot and spring
- ☐ Vise arms and adjusting chain
- ☐ Motor and drive shaft

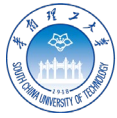

**4. What are the vise jaws and movable jaws of a bench vise typically made of?**

- ☐ Plastic
- ☐ Wood
- ☐ Metal
- ☐ Rubber

**5. What is the purpose of the vise seat in a bench vise?**

- ☐ Securing the body
- ☐ Clamping objects
- ☐ Adjusting the jaw width
- ☐ Adjusting the opening degree

**6. What is the function of a pin?**

- ☐ Securing nuts
- ☐ Securing the vise seat
- ☐ Preventing nuts from loosening and coming off
- ☐ Adjusting the jaw width

**7. What is the function of a nut?**

- ☐ Securing nuts
- ☐ Securing the vise seat
- ☐ Preventing the screw from loosening and coming out
- ☐ Adjusting the jaw width

**8. What can a bench vise be used to clamp?**

- ☐ Metal materials
- ☐ Wood and plastic
- ☐ Electronic components
- ☐ All objects

**10. Please write the corresponding names for the numbered labels below:**

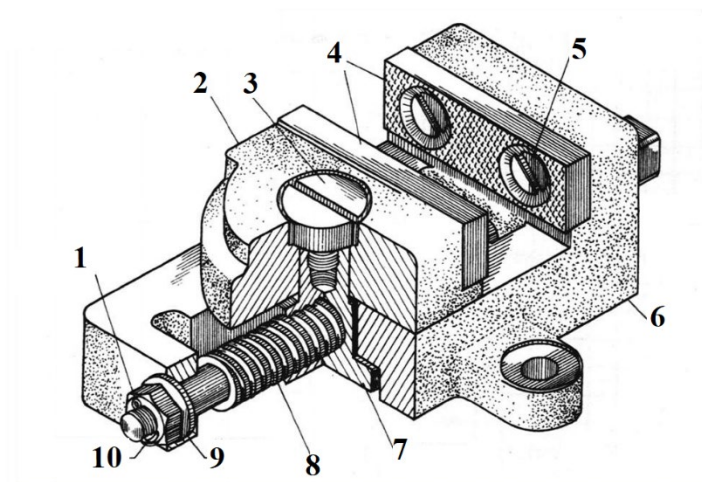

Supplement: Supplementary file 1 [file Appendix1_pre_test.pdf]
