# Supplementary material for: Measuring the Sense of Presence and Learning Efficacy in Immersive Virtual Assembly Training
Source: arXiv:2312.10387 source file (2023-12-16)
Supplement: Supplementary file 2 [file Appendix2_scale.pdf]

## Appendix II

### Scale for Assessing Subjects' Subjective Sensations

| #   | Fac. | Question                                                  | Evaluation |
|-----|------|-----------------------------------------------------------|------------|
| Q01 | CF   | No perceived delay between actions and expected outcomes. | 1 □□□□□□ 7 |
| Q02 | CF   | Frequent interaction with virtual elements.               | 1 □□□□□□ 7 |
| Q03 | CF   | Able to move and manipulate objects in VR.                | 1 □□□□□□ 7 |
| Q04 | CF   | System responds adequately to actions.                    | 1 □□□□□□ 7 |
| Q05 | CF   | Feedback from app operations as expected.                 | 1 □□□□□□ 7 |
| Q06 | CF   | Feedback from device operations as expected.              | 1 □□□□□□ 7 |
| Q07 | CF   | Natural feeling during app interaction.                   | 1 □□□□□□ 7 |
| Q08 | CF   | Natural feeling during device operation.                  | 1 □□□□□□ 7 |
| Q09 | CF   | No complex issues encountered in app use.                 | 1 □□□□□□ 7 |
| Q10 | CF   | No complex issues encountered with device.                | 1 □□□□□□ 7 |
| Q11 | CF   | App usage is easy.                                        | 1 □□□□□□ 7 |
| Q12 | CF   | Device operation is easy.                                 | 1 □□□□□□ 7 |
| Q13 | CF   | Sense of control over virtual events.                     | 1 □□□□□□ 7 |
| Q14 | CF   | Quick adaptation to VR environment.                       | 1 □□□□□□ 7 |
| Q15 | CF   | Proficient in VR interaction by the end.                  | 1 □□□□□□ 7 |
| Q16 | SF   | Clear information in the virtual environment.             | 1 □□□□□□ 7 |
| Q17 | SF   | Full sensory engagement in the task.                      | 1 □□□□□□ 7 |
| Q18 | SF   | Level of immersion through visuals.                       | 1 □□□□□□ 7 |
| Q19 | SF   | Level of immersion through auditory cues.                 | 1 □□□□□□ 7 |
| Q20 | SF   | Perception of object movements in VR.                     | 1 □□□□□□ 7 |
| Q21 | SF   | Active search for virtual targets.                        | 1 □□□□□□ 7 |
| Q22 | SF   | Sensation of movement within VR.                          | 1 □□□□□□ 7 |
| Q23 | SF   | Careful examination of virtual objects.                   | 1 □□□□□□ 7 |
| Q24 | SF   | Examination of objects from multiple angles.              | 1 □□□□□□ 7 |
| Q25 | SF   | Consistent information across senses.                     | 1 □□□□□□ 7 |
| Q26 | SF   | Consistent experience across senses.                      | 1 □□□□□□ 7 |
| Q27 | DF   | Focus on task actions, not system/environment.            | 1 □□□□□□ 7 |
| Q28 | DF   | Awareness of real-world events during the task.           | 1 □□□□□□ 7 |
| Q29 | DF   | Good understanding of the device.                         | 1 □□□□□□ 7 |
| Q30 | DF   | Device operation doesn't distract from the task.          | 1 □□□□□□ 7 |
| Q31 | DF   | Visual interface doesn't distract from the task.          | 1 □□□□□□ 7 |
| Q32 | DF   | Helpful guiding elements in VR.                           | 1 □□□□□□ 7 |
| Q33 | DF   | Appreciation for helpful guiding elements.                | 1 □□□□□□ 7 |
| Q34 | RF   | High realism of the virtual environment.                  | 1 □□□□□□ 7 |
| Q35 | RF   | Occasional confusion between virtual and real.            | 1 □□□□□□ 7 |

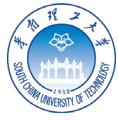

| #   | Fac. | Question                                         | Evaluation |
|-----|------|--------------------------------------------------|------------|
| Q36 | RF   | Feeling of touch in the virtual environment.     | 1 □□□□□□ 7 |
| Q37 | RF   | VR experience consistent with real-world.        | 1 □□□□□□ 7 |
| Q38 | RF   | Slight disappointment at rest/experiment end.    | 1 □□□□□□ 7 |
| Q39 | RF   | Improved understanding of structures after task. | 1 □□□□□□ 7 |
| Q40 | EF   | No discomfort (dizziness) during experience.     | 1 □□□□□□ 7 |
| Q41 | EF   | User-friendly for limbs.                         | 1 □□□□□□ 7 |
| Q42 | EF   | User-friendly for head and neck.                 | 1 □□□□□□ 7 |
| Q43 | EF   | User-friendly for eyes, ears, nose, mouth.       | 1 □□□□□□ 7 |
| Q44 | EF   | No mental pressure during device use.            | 1 □□□□□□ 7 |
