# Supplementary material for: Measuring the Sense of Presence and Learning Efficacy in Immersive Virtual Assembly Training
Source: arXiv:2312.10387 source file (2023-12-16)

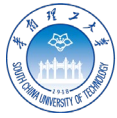

## Appendix III: Post-test

Name \_\_\_\_\_ Gender \_\_\_\_\_  
Age \_\_\_\_\_ Studies \_\_\_\_\_

[ Mark with an X the box you consider correct ]

**1. What is the primary function of a bench vise?**

- ☐ Loosening bolts
- ☐ Clamping objects
- ☐ Twisting objects
- ☐ Cutting objects

**2. What are the components of a bench vise?**

- ☐ Vise seat, movable jaws, screws, gears
- ☐ Seat, washers, screws, jaws
- ☐ Vise seat, washers, gears, handle
- ☐ Vise seat, washers, screws, cutting blades

**3. What is the working principle of a bench vise?**

- ☐ Adjusting the jaw opening by rotating the nut
- ☐ Deforming objects by squeezing them
- ☐ Controlling jaw opening and clamping force through the action of the vise jaws and vise seat, thereby gripping and securing objects
- ☐ Adjusting the clamping force by rotating the jaw plates

**4. If you need to increase the clamping force of a bench vise, how should you adjust it?**

- ☐ Adjusting by rotating the nut
- ☐ Replacing the jaw plates
- ☐ Adding washers
- ☐ Adjusting it through the screw

**5. What is the main application area of a bench vise?**

- ☐ Metalworking
- ☐ Woodworking
- ☐ Textile manufacturing
- ☐ Machine repair

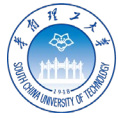

**6. What is the function of the bench vise pad?**

- ☐ To adjust the opening size
- ☐ To adjust the clamping force
- ☐ To protect the vise jaw from damage
- ☐ To increase the width of the vise jaws

**7. What is the working principle of a bench vise based on?**

- ☐ Lever principle
- ☐ Hydraulic principle
- ☐ Electric principle
- ☐ Magnetic principle

**8. Which of the following is NOT a component of a bench vise?**

- ☐ Spindle
- ☐ Helical spring
- ☐ Base
- ☐ Pad

**8. Which of the following is NOT a component of a bench vise?**

- ☐ Spindle
- ☐ Helical spring
- ☐ Base
- ☐ Pad

**9. What type of motion enables the linear movement of the movable jaw of a bench vise?**

- ☐ Rotary motion
- ☐ Angular motion
- ☐ Helical motion
- ☐ Radial motion

**10. What is the function of the square nut on a bench vise?**

- ☐ To transfer torque
- ☐ To control the width of the jaws
- ☐ To adjust the clamping force
- ☐ To enable linear motion of the movable jaw

**11. What is a bench vise used for on a machine shop workbench?**

- ☐ To clamp workpieces for machining
- ☐ To fix the machine shop workbench
- ☐ For cleaning work
- ☐ To measure the precision of the machine shop workbench

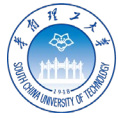

**12. How does a bench vise clamp a workpiece?**

- ☐ Through the rotation of the movable jaw
- ☐ Through the linear motion of the movable jaw
- ☐ Through the rotation of the square nut
- ☐ None of the above

**13. What is the function of the nut on a bench vise?**

- ☐ To fix the nut
- ☐ To fix the vise base
- ☐ To prevent the screw from loosening and slipping out
- ☐ To adjust the width of the jaws

**14. What is the function of the pin on a bench vise??**

- ☐ Through the rotation of the movable jaw
- ☐ Through the linear motion of the movable jaw
- ☐ Through the rotation of the square nut
- ☐ None of the above

**15. What is the vise seat of a bench vise used for?**

- ☐ To fix the vise body
- ☐ To clamp objects
- ☐ To prevent the nut from loosening and slipping out
- ☐ To adjust the width of the jaws

**16. What materials are the jaws of a bench vise typically made of?**

- ☐ Metal
- ☐ Wood
- ☐ Plastic
- ☐ Rubber

**17. What components can be used to adjust the clamping force and opening width of a bench vise?**

- ☐ Pins, nuts, screws, and washers
- ☐ Pivot axis and springs
- ☐ Arms and chains
- ☐ Motor and drive shaft

**18. Where are bench vises commonly used on machine tools?**

- ☐ Milling machines
- ☐ Drill presses
- ☐ Lathes
- ☐ All of the above

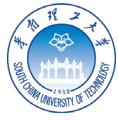

**19. What component drives the movable jaw of a bench vise to move?**

- ☐ Belt drive
- ☐ Square nut
- ☐ Crankshaft linkage
- ☐ Hydraulic cylinder

**20. How does a bench vise operate, and which components are involved?**

- ☐ Base and seat
- ☐ Jaws and washers
- ☐ Movable jaw and pins
- ☐ Nut and screw

**21. Please write the corresponding names for the numbered labels below:**

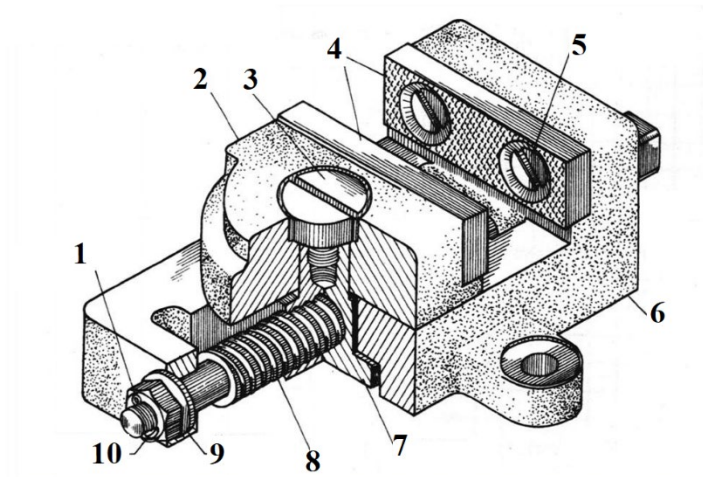

Supplement: Supplementary file 3 [file Appendix3_post_test.pdf]
